# Supplementary material for: Machine learning surrogate models for particle insertions and element substitutions
Source: arXiv:2409.19188 ancillary file (2024-10-04)
Supplement: Supplementary file 1 [file supplementary_information.pdf]

# Supplementary Information for machine learning surrogate models for particle insertions and element substitutions

Ryosuke Jinnouchi

*Toyota Central R&D Labs., Inc., 41-1 Yokomichi, Nagakute, Aichi, 480-1192, Japan*

(Dated: September 28, 2024)

Table S 1. Parameter sets of descriptors and kernel basis functions.

| | | | | | |
|---|---|---|---|---|---|
| $\zeta$ 4 | $\beta^{(2)}$ 0.5 | $R_{\mathrm{cut}}^{(2)}$ 6.0 | $\sigma_{\mathrm{atom}}^{(2)}$ 0.5 | $N_{\mathrm{R}}^{(2)}$ 8 | |
| | $\beta^{(3)}$ 0.5 | $R_{\mathrm{cut}}^{(3)}$ 4.0 | $\sigma_{\mathrm{atom}}^{(3)}$ 0.5 | $N_{\mathrm{R}}^{(3)}$ 6 | $L_{\max}^{(3)}$ 3 |

Table S 2. The averaged value of 1s levels of oxygen atoms at the middle of the water slab, scaled to the electrostatic potential in the vacuum layer ($\varepsilon_{\mathrm{1s,slab}} - \mu$), in the same system, and the one in the region far from the ions in the bulk liquids, scaled to the average electrostatic potential in the same system ($\varepsilon_{\mathrm{1s,bulk}}$). The potential gaps $e\Delta\phi = \mu - \varepsilon_{\mathrm{1s,slab}} + \varepsilon_{\mathrm{1s,bulk}}$ for the bulk liquids are also shown. Units are in eV.

| System | $\varepsilon_{\mathrm{1s,slab}} - \mu$ | |
|---|---|---|
| $128H_2O$ slab | −511.23±0.02 | |
| System | $\varepsilon_{\mathrm{1s,bulk}}$ | $e\Delta\phi$ |
| $64H_2O$ | −507.59±0.00 | 3.64±0.02 |
| $H^+$+$64H_2O$ | −507.52±0.01 | 3.71±0.02 |
| $Li^+$+$64H_2O$ | −507.58±0.00 | 3.65±0.02 |
| $Na^+$+$64H_2O$ | −507.55±0.00 | 3.68±0.02 |
| $K^+$+$64H_2O$ | −507.52±0.00 | 3.71±0.02 |
| $Rb^+$+$64H_2O$ | −507.50±0.00 | 3.73±0.02 |
| $Cs^+$+$64H_2O$ | −507.44±0.00 | 3.79±0.02 |
| $Fr^+$+$64H_2O$ | −507.44±0.00 | 3.80±0.02 |
| $F^-$+$64H_2O$ | −507.54±0.00 | 3.69±0.02 |
| $Cl^-$+$64H_2O$ | −507.49±0.00 | 3.74±0.02 |
| $Br^-$+$64H_2O$ | −507.48±0.00 | 3.75±0.02 |
| $I^-$+$64H_2O$ | −507.41±0.00 | 3.82±0.02 |
| $At^-$+$64H_2O$ | −507.40±0.00 | 3.84±0.02 |

Table S 3. Real potentials of single ions computed by the particle insertion and element substitution methods. Unit is eV.

| Particle insertion | | | | Element substitution | | | |
|---|---|---|---|---|---|---|---|
| Cation | | Anion | | Cation | | Anion | |
| $H^+$ | −10.98±0.05 | | | $H^+$ | −11.01±0.09 | | |
| $Li^+$ | −5.07±0.07 | $F^-$ | −4.65±0.05 | $Li^+$ | −5.05±0.09 | $F^-$ | −4.68±0.08 |
| $Na^+$ | −4.01±0.07 | $Cl^-$ | −3.37±0.08 | $Na^+$ | −3.99±0.10 | $Cl^-$ | −3.38±0.06 |
| $K^+$ | −3.22±0.09 | $Br^-$ | −3.11±0.05 | $K^+$ | −3.22±0.10 | $Br^-$ | −3.17±0.07 |
| $Rb^+$ | −2.97±0.08 | $I^-$ | −2.71±0.07 | $Rb^+$ | −2.94±0.09 | $I^-$ | −2.69±0.06 |
| $Cs^+$ | −2.65±0.11 | $At^-$ | −2.58±0.06 | $Cs^+$ | −2.65±0.09 | $At^-$ | −2.59±0.07 |
| $Fr^+$ | −2.58±0.08 | | | $Fr^+$ | −2.57±0.11 | | |

Table S 4. Peak positions and the number of water molecules in the first and second solvation shells of cations obtained by the MLFFs compared with previous reports. Symbols $r_1$ and $r_2$ denote the positions of the maximum points of the first and second peaks, respectively, in the RDF between the ion and oxygen atoms in water molecules. Symbols $n_1$ and $n_2$ denote the numbers of water molecules in the first and second solvation shells, respectively. Here, the first solvation shell is defined as the region from the origin to the first minimum of the RDF, and the second solvation shell is defined as the region from the first minimum to the second minimum similar to the previous studies. Values in parentheses and square brackets are the simulated and experimental results from past studies. Because the second minima for $Rb^+$, $Cs^+$, and $Fr^+$ were large relative to the cell size, their relevant values were not determined.

| | $r_1$ | $n_1$ | $r_2$ | $n_2$ |
|---|---|---|---|---|
| $H_3O^+$ | 2.52 | 3.2 | 4.14 | 18.4 |
| | (2.50-2.51)[a] | (3)[a] | (4.3)[a] | |
| $Li^+$ | 1.98 | 4.1 | 4.00 | 19.7 |
| | (1.96)[b] | (4,-4.1)[b] | (4.28)[b] | (16)[c] |
| | [1.94-2.07][d] | | | |
| $Na^+$ | 2.47 | 6.2 | 4.54 | 24.0 |
| | (2.37-2.49)[e] | (5.2-6.1)[e] | (4.2-4.5)[e] | (16-18.3)[e] |
| | [2.39][f] | [4-6][f] | | |
| $K^+$ | 2.91 | 8.3 | 4.98 | 18.5 |
| | (2.74-2.87)[g] | (6.7-7.9)[g] | (4.84)[g] | (16-18.3)[g] |
| | [2.81][h] | [4-7][h] | | |
| $Rb^+$ | 3.11 | 8.2 | 5.03 | 21.2 |
| | (2.92)[i] | (8.0)[i] | 5.04[i] | 20.7[i] |
| | [2.9-2.98][j] | [6-8][j] | | |
| $Cs^+$ | 3.27 | 21.6 | | |
| | (3.15)[i] | (9.6)[i] | | |
| | [2.9-3.07][k] | [8.0][k] | | |
| $Fr^+$ | 3.33 | 22.3 | | |

a. Simulations using the BLYP functional from Ref. [1, 2].

b. Simulations using the BLYP functional from Ref. [3].

c. Simulations using polarizable force fields from Ref. [4].

d. X-ray and neutron scattering measurements in Ref. [5–8].

e. Simulations using a polarizable force field in Ref. [4] and BLYP, HCTH and PBE functionals with and without the dispersion correction in Ref. [9, 10].

f. X-ray scattering measurements in Ref. [8, 11–13].

g. Simulations using polarizable force fields in Ref. [4, 14] and BLYP, HCTH and PBE functionals with and without the dispersion correction in Ref. [10, 15].

h. X-ray scattering in Ref. [8].

i. Simulations using polarizable force fields in Ref. [4].

j. X-ray absorption, and X-ray and neutron scattering measurements in Ref. [8, 16–18].

k. X-ray and neutron scattering measurements in Ref. [8].

Table S 5. Peak positions and the number of water molecules in the first and second solvation shells of anions obtained by the RPBE+D3 functional compared with previous reports. The meanings of the symbols are the same as those in Table 5. Because the second minima for $Br^-$, $I^-$, and $At^-$ were large relative to the cell size, their relevant values were not determined.

| | $r_1$ | $n_1$ | $r_2$ | $n_2$ |
|---|---|---|---|---|
| $F^-$ | 2.71 | 5.3 | 4.72 | 21.2 |
| | (2.66-2.69)[a] | (4.6-5.7)[a] | (4.61)[b] | (20.0)[b] |
| | [2.6-2.9][c] | [4-6][c] | | |
| $Cl^-$ | 3.20 | 6.4 | 5.23 | 23.2 |
| | (3.14-3.19)[a] | (5.9-6.6)[a] | (4.88)[b] | (23.3)[b] |
| | [3.1-3.3][c] | [4-9][c] | | |
| $Br^-$ | 3.37 | 7.0 | | |
| | (3.26-3.27)[d] | 6.6[d] | | |
| | [3.19-3.4][e] | 6.0-7.4[e] | | |
| $I^-$ | 3.60 | 13.5 | | |
| | (3.49-3.55)[f] | 6.7-9.7[f] | | |
| | [3.60-3.76][g] | 6.0-8.8[g] | | |
| $At^-$ | 3.75 | 17.7 | | |

a. Simulations using a polarizable force field in Ref. [4], QM/MM in Ref. [19] and BLYP functional in Ref, [20].

b. Simulations using a polarizable force field in Ref. [4].

c. Neutron and X-ray scattering measurements in Ref. [21, 22].

d. Simulations using a polarizable force field in Ref. [4] and BLYP functional in Ref. [23, 24].

e. X-ray absorption measurements in Ref. [18, 25–30].

f. Simulations using conventional force fields in Ref. [4, 31–36] and BLYP functional in Ref. [37].

g. X-ray absorption and scattering measurements in Ref. [38, 39].

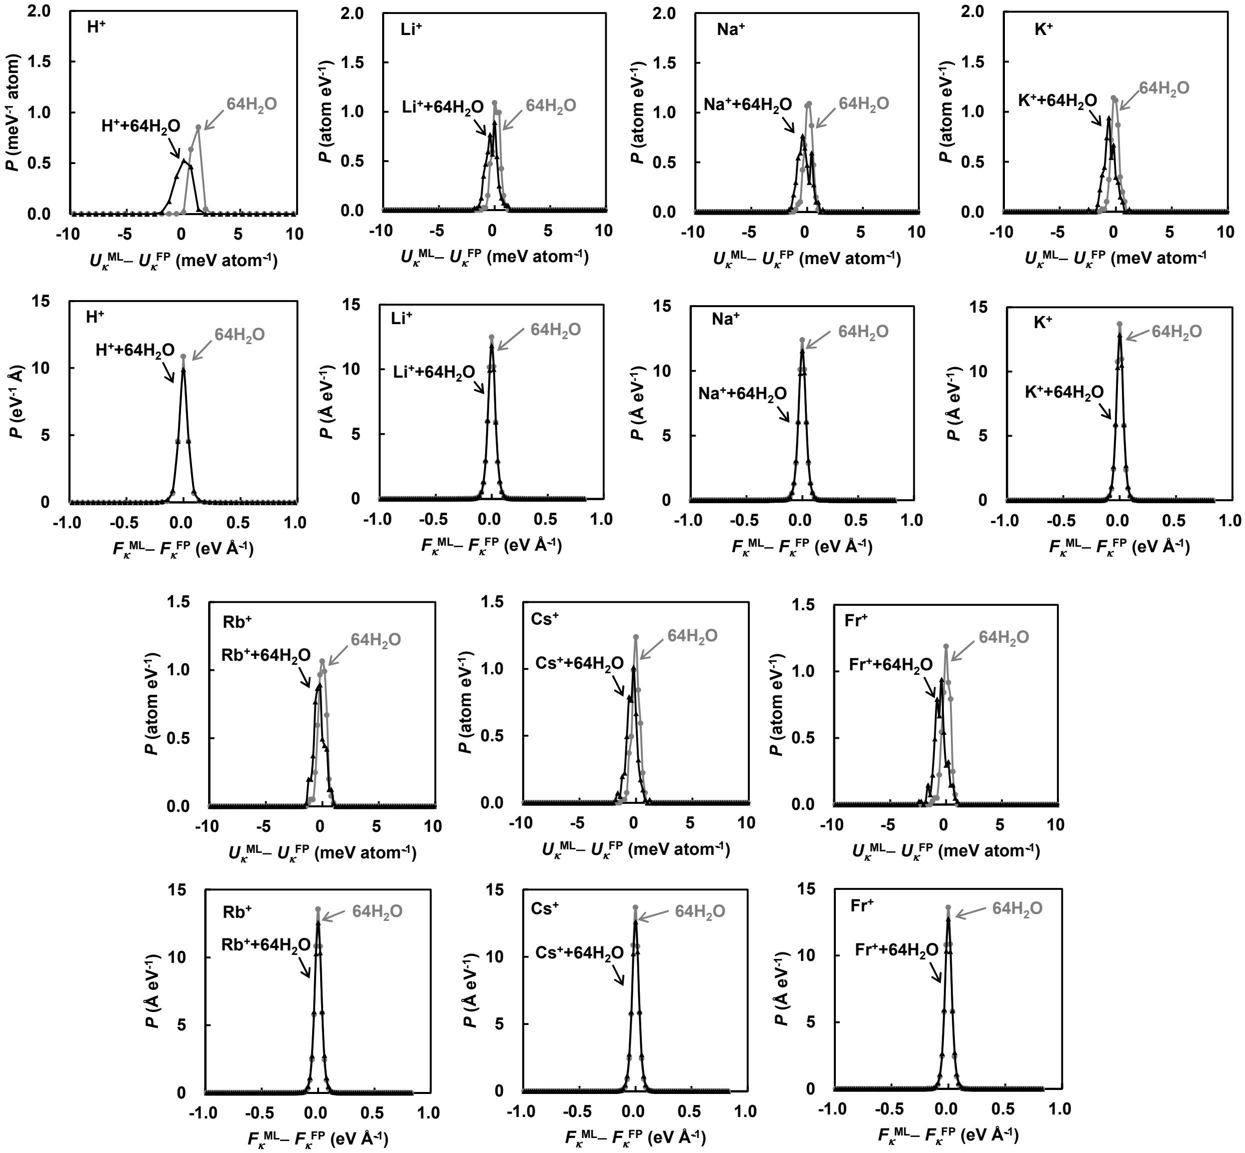


Figure S 1. Error distributions of energies ($U_\kappa^{\mathrm{ML}}$) and forces ($F_\kappa^{\mathrm{ML}}$) for the systems before ($\kappa$=0) and after ($\kappa$=1) the particle insertions, as predicted by the MLFFs used for the cation insertion calculations, compared with the FP results ($U_\kappa^{\mathrm{FP}}$ and $F_\kappa^{\mathrm{FP}}$).

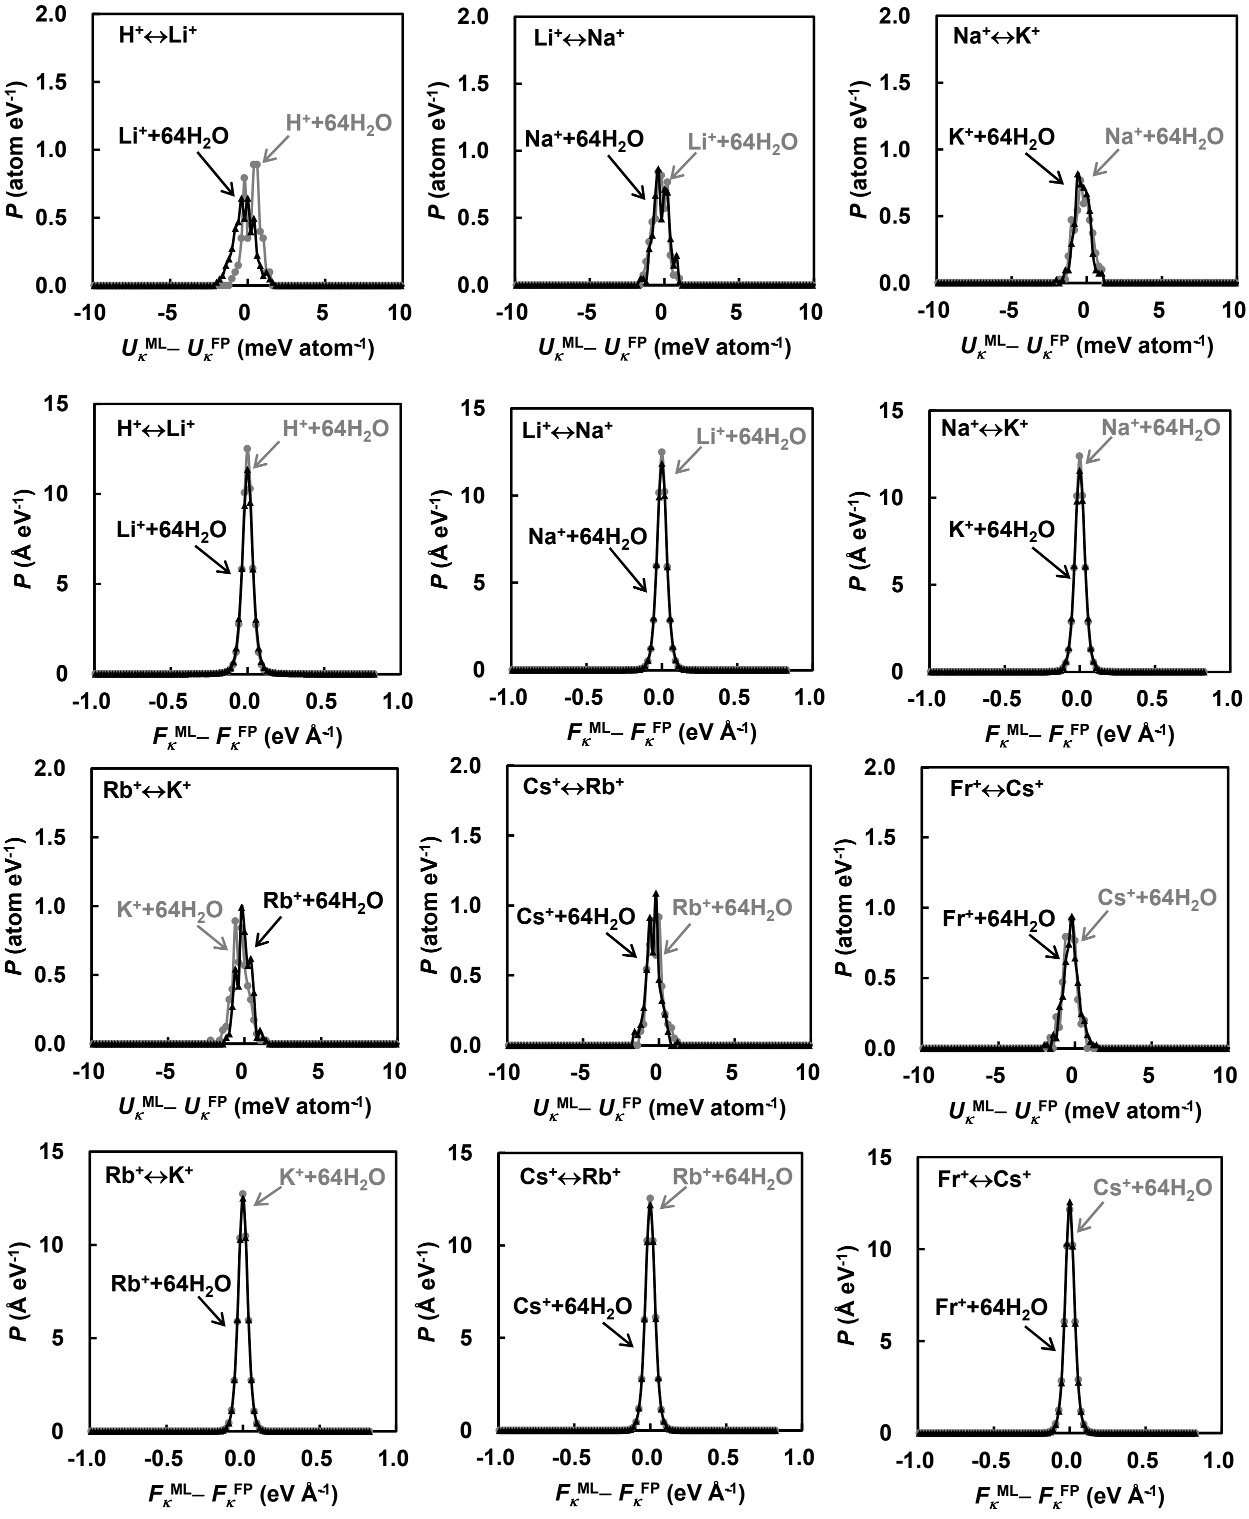


Figure S 2. Error distributions of energies ($U_{\kappa}^{\mathrm{ML}}$) and forces ($F_{\kappa}^{\mathrm{ML}}$) for the systems before ($\kappa$=0) and after ($\kappa$=1) the element substitutions, as predicted by the MLFFs used for the cation substitution calculations, compared with the FP results ($U_{\kappa}^{\mathrm{FP}}$ and $F_{\kappa}^{\mathrm{FP}}$).

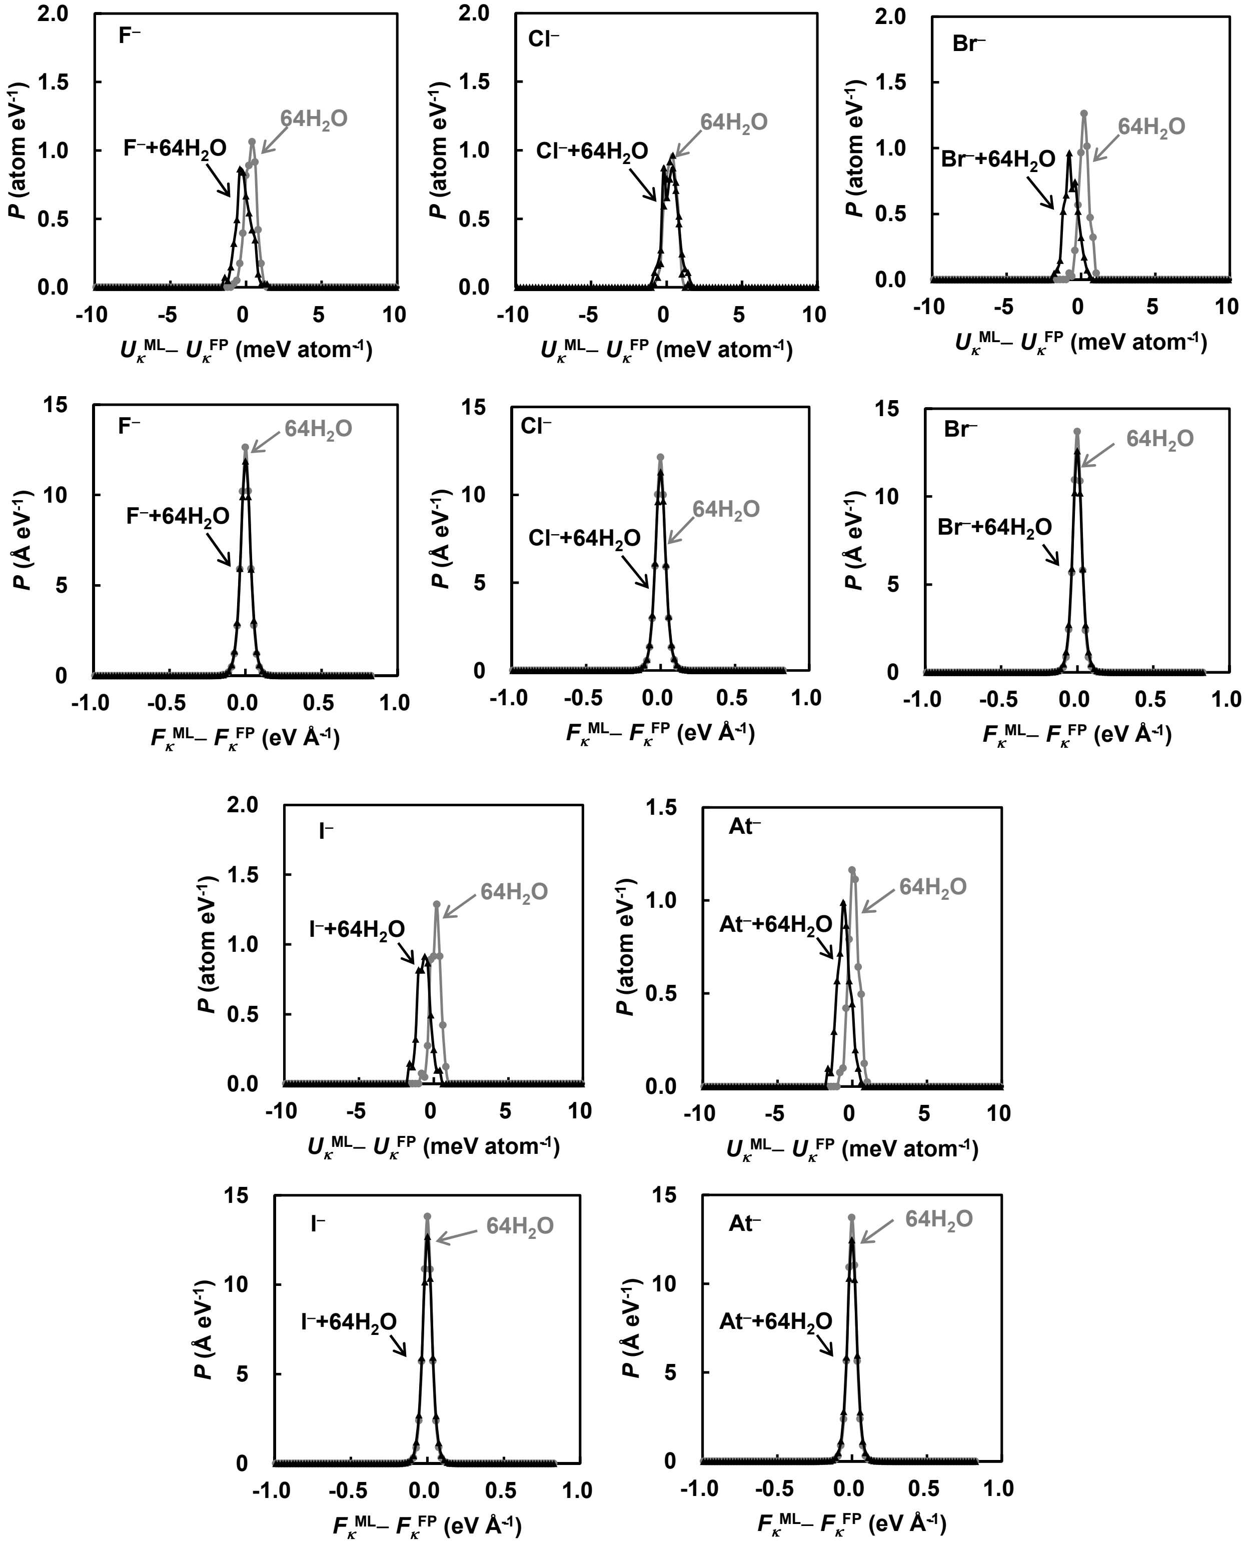


Figure S 3. Error distributions of energies ($U_{\kappa}^{\mathrm{ML}}$) and forces ($F_{\kappa}^{\mathrm{ML}}$) for the systems before ($\kappa$=0) and after ($\kappa$=1) the anion substitutions, as predicted by the MLFFs used for the anion insertion calculations, compared with the FP results ($U_{\kappa}^{\mathrm{FP}}$ and $F_{\kappa}^{\mathrm{FP}}$).

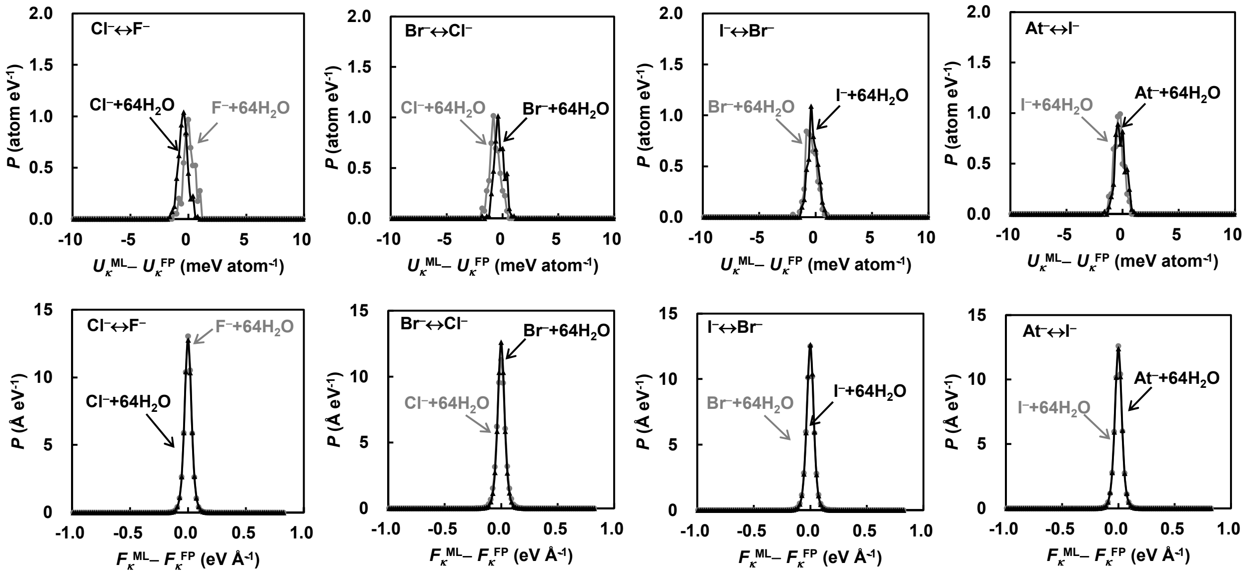


Figure S 4. Error distributions of energies ($U_{\kappa}^{\mathrm{ML}}$) and forces ($F_{\kappa}^{\mathrm{ML}}$) for the systems before ($\kappa$=0) and after ($\kappa$=1) the element substitutions, as predicted by the MLFFs used for the anion substitution calculations, compared with the FP results ($U_{\kappa}^{\mathrm{FP}}$ and $F_{\kappa}^{\mathrm{FP}}$).

[1] M. Tuckerman, K. Laasonen, M. Sprik, and M. Parrinello. Ab initio molecular dynamics simulation of the solvation and transport of hydronium and hydroxyl ions in water. *The Journal of Chemical Physics*, 103(1):150–161, 07 1995.

[2] Sergei Izvekov and Gregory A. Voth. Ab initio molecular-dynamics simulation of aqueous proton solvation and transport revisited. *The Journal of Chemical Physics*, 123(4):044505, 08 2005.

[3] A. P. Lyubartsev, K. Laasonen, and A. Laaksonen. Hydration of $Li^+$ ion. An ab initio molecular dynamics simulation. *The Journal of Chemical Physics*, 114(7):3120–3126, 02 2001.

[4] Guillaume Lamoureux and Benoît Roux. Absolute hydration free energy scale for alkali and halide ions established from simulations with a polarizable force field. *The Journal of Physical Chemistry B*, 110(7):3308–3322, Feb 2006.

[5] A. Musinu, G. Paschina, G. Piccaluga, and M. Magini. X-ray diffraction study of $CoCl_2$–LiCl aqueous solutions. *The Journal of Chemical Physics*, 80(6):2772–2776, 03 1984.

[6] A. P. Copestake, G. W. Neilson, and J. E. Enderby. The structure of a highly concentrated aqueous solution of lithium chloride. *Journal of Physics C: Solid State Physics*, 18(22):4211, Aug 1985.

[7] T Cartailler, W Kunz, P Turq, and M C Bellisent-Funel. Lithium bromide in acetonitrile and water: a neutron scattering study. *Journal of Physics: Condensed Matter*, 3(47):9511, nov 1991.

[8] Johan Mähler and Ingmar Persson. A study of the hydration of the alkali metal ions in aqueous solution. *Inorganic Chemistry*, 51(1):425–438, Jan 2012.

[9] Jody A. White, Eric Schwegler, Giulia Galli, and François Gygi. The solvation of $Na^+$ in water: First-principles simulations. *The Journal of Chemical Physics*, 113(11):4668–4673, 09 2000.

[10] Arindam Bankura, Vincenzo Carnevale, and Michael L. Klein. Hydration structure of salt solutions from ab initio molecular dynamics. *The Journal of Chemical Physics*, 138(1):014501, 01 2013.

[11] R. Caminiti, G. Licheri, G. Paschina, G. Piccaluga, and G. Pinna. Interactions and structure in aqueous $NaNO_3$ solutions. *The Journal of Chemical Physics*, 72(8):4522–4528, 04 1980.

[12] N T Skipper and G W Neilson. X-ray and neutron diffraction studies on concentrated aqueous solutions of sodium nitrate and silver nitrate. *Journal of Physics: Condensed Matter*, 1(26):4141, jul 1989.

[13] Yasuo Kameda, Kentaro Sugawara, Takeshi Usuki, and Osamu Uemura. Hydration Structure of $Na^+$ in Concentrated Aqueous Solutions. *Bulletin of the Chemical Society of Japan*, 71(12):2769–2776, 06

2006.

[14] Alan Grossfield, Pengyu Ren, and Jay W. Ponder. Ion solvation thermodynamics from simulation with a polarizable force field. *Journal of the American Chemical Society*, 125(50):15671–15682, Dec 2003.

[15] Lavanya M. Ramaniah, Marco Bernasconi, and Michele Parrinello. Ab initio molecular-dynamics simulation of $K^+$ solvation in water. *The Journal of Chemical Physics*, 111(4):1587–1591, 07 1999.

[16] Johan E. Enderby. Ion solvation via neutron scattering. *Chem. Soc. Rev.*, 24:159–168, 1995.

[17] J. L. Fulton, D. M. Pfund, S. L. Wallen, M. Newville, E. A. Stern, and Yanjun Ma. Rubidium ion hydration in ambient and supercritical water. *The Journal of Chemical Physics*, 105(6):2161–2166, 08 1996.

[18] Adriano Filipponi, Simone De Panfilis, Cecilia Oliva, Maria Antonietta Ricci, Paola D'Angelo, and Daniel T. Bowron. Ion hydration under pressure. *Phys. Rev. Lett.*, 91:165505, Oct 2003.

[19] Anan Tongraar and Bernd Michael Rode. The hydration structures of $F^-$ and $Cl^-$ investigated by ab initio qm/mm molecular dynamics simulations. *Phys. Chem. Chem. Phys.*, 5:357–362, 2003.

[20] J. M. Heuft and E. J. Meijer. Density functional theory based molecular-dynamics study of aqueous fluoride solvation. *The Journal of Chemical Physics*, 122(9):094501, 02 2005.

[21] G. W. Neilson and R. H. Tromp. Chapter 3. neutron and X-ray diffraction on aqueous solutions. *Annu. Rep. Prog. Chem., Sect. C: Phys. Chem.*, 88:45–75, 1991.

[22] Hitoshi. Ohtaki and Tamas. Radnai. Structure and dynamics of hydrated ions. *Chemical Reviews*, 93(3):1157–1204, May 1993.

[23] Simone Raugei and Michael L. Klein. Dynamics of water molecules in the $Br^-$ solvation shell: an ab initio molecular dynamics study. *Journal of the American Chemical Society*, 123(38):9484–9485, Sep 2001.

[24] Paola D'Angelo, Valentina Migliorati, and Leonardo Guidoni. Hydration properties of the bromide aqua ion: the interplay of first principle and classical molecular dynamics, and X-ray absorption spectroscopy. *Inorganic Chemistry*, 49(9):4224–4231, May 2010.

[25] P. D'Angelo, A. Di Nola, A. Filipponi, N. V. Pavel, and D. Roccatano. An extended X-ray absorption fine structure study of aqueous solutions by employing molecular dynamics simulations. *The Journal of Chemical Physics*, 100(2):985–994, 01 1994.

[26] Hajime Tanida, Hideto Sakane, and Iwao Watanabe. Solvation structures for bromide ion in various solvents by extended X-ray absorption fine structure. *J. Chem. Soc., Dalton Trans.*, pages 2321–2326,

1994.

[27] R. Beudert, H. Bertagnolli, and M. Zeller. Ion–ion and ion–water interactions in an aqueous solution of erbium bromide ($ErBr_3$). A differential anomalous x-ray scattering study. *The Journal of Chemical Physics*, 106(21):8841–8848, 06 1997.

[28] Scott L. Wallen, Bruce J. Palmer, David M. Pfund, John L. Fulton, Matthew Newville, Yanjun Ma, and Edward A. Stern. Hydration of bromide ion in supercritical water: an X-ray absorption fine structure and molecular dynamics study. *The Journal of Physical Chemistry A*, 101(50):9632–9640, Dec 1997.

[29] G. Ferlat, A. San Miguel, J. F. Jal, J. C. Soetens, Ph. A. Bopp, I. Daniel, S. Guillot, J. L. Hazemann, and R. Argoud. Hydration of the bromine ion in a supercritical 1:1 aqueous electrolyte. *Phys. Rev. B*, 63:134202, Mar 2001.

[30] D T Bowron. Comprehensive structural modelling of aqueous solutions using neutron diffraction and X-ray absorption spectroscopy. *Journal of Physics: Conference Series*, 190(1):012022, nov 2009.

[31] Liem X. Dang and Bruce C. Garrett. Photoelectron spectra of the hydrated iodine anion from molecular dynamics simulations. *The Journal of Chemical Physics*, 99(4):2972–2977, 08 1993.

[32] Song Hi Lee and Jayendran C. Rasaiah. Molecular dynamics simulation of ion mobility. 2. alkali metal and halide ions using the SPC/E model for water at 25 °c. *The Journal of Physical Chemistry*, 100(4):1420–1425, Jan 1996.

[33] Gergely Tóth. Ab initio pair potential parameter set for the interaction of a rigid and a flexible water model and the complete series of the halides and alkali cations. *The Journal of Chemical Physics*, 105(13):5518–5524, 10 1996.

[34] S. Koneshan, Jayendran C. Rasaiah, R. M. Lynden-Bell, and S. H. Lee. Solvent structure, dynamics, and ion mobility in aqueous solutions at 25 °c. *The Journal of Physical Chemistry B*, 102(21):4193–4204, May 1998.

[35] Barbara Hribar, Noel T. Southall, Vojko Vlachy, and Ken A. Dill. How ions affect the structure of water. *Journal of the American Chemical Society*, 124(41):12302–12311, Oct 2002.

[36] Regla Ayala, José M. Martínez, Rafael R. Pappalardo, and Enrique Sánchez Marcos. On the halide hydration study: Development of first-principles halide ion-water interaction potential based on a polarizable model. *The Journal of Chemical Physics*, 119(18):9538–9548, 11 2003.

[37] J. M. Heuft and E. J. Meijer. Density functional theory based molecular-dynamics study of aqueous iodide solvation. *The Journal of Chemical Physics*, 123(9):094506, 09 2005.

[38] Richard M. Lawrence and R. F. Kruh. X-Ray Diffraction Studies of Aqueous Alkali-Metal Halide

Solutions. *The Journal of Chemical Physics*, 47(11):4758–4765, 12 1967.

[39] Alfred H. Narten. Diffraction pattern and structure of aqueous ammonium halide solutions. *The Journal of Physical Chemistry*, 74(4):765–768, Feb 1970.
